# Supplementary material for: Revisiting ab-initio excited state forces from many-body Green's function formalism: approximations and benchmark
Source: arXiv:2502.05144 source file (2026-08-15)

band 1

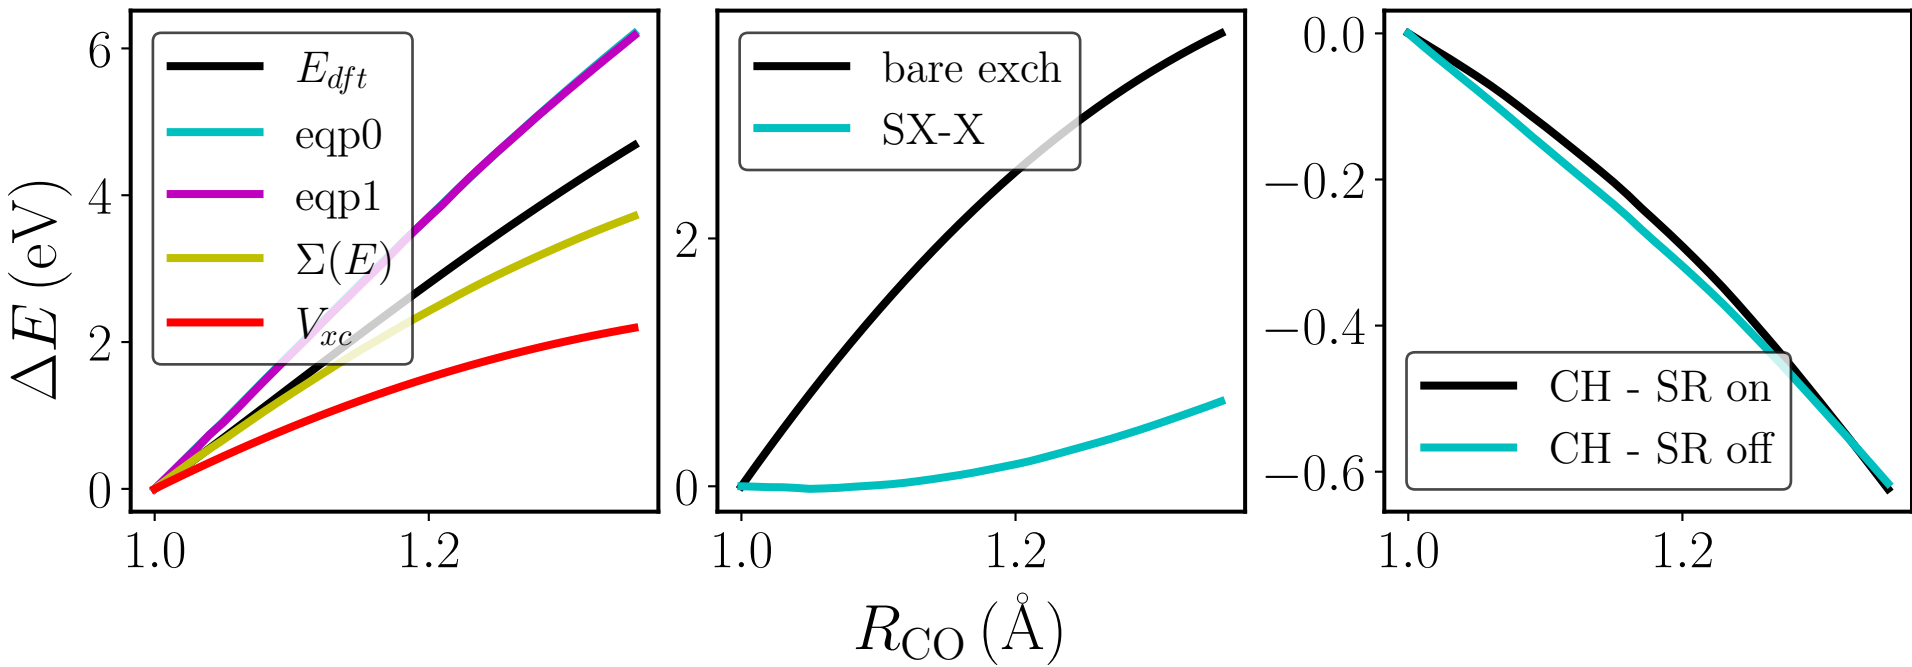

# band 2

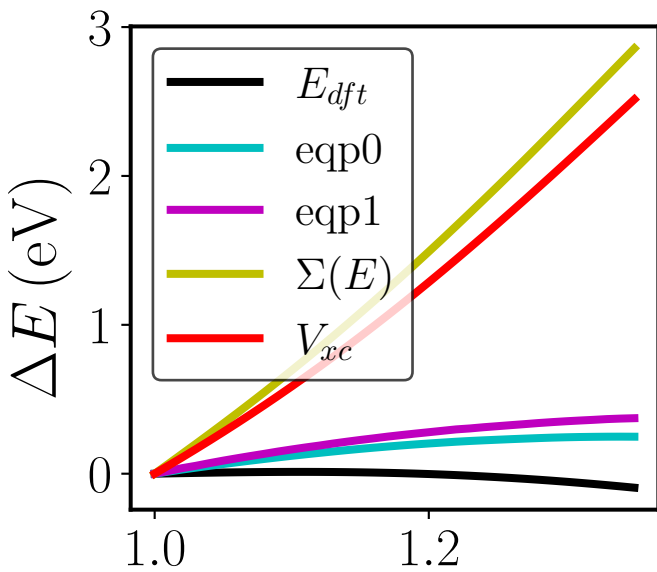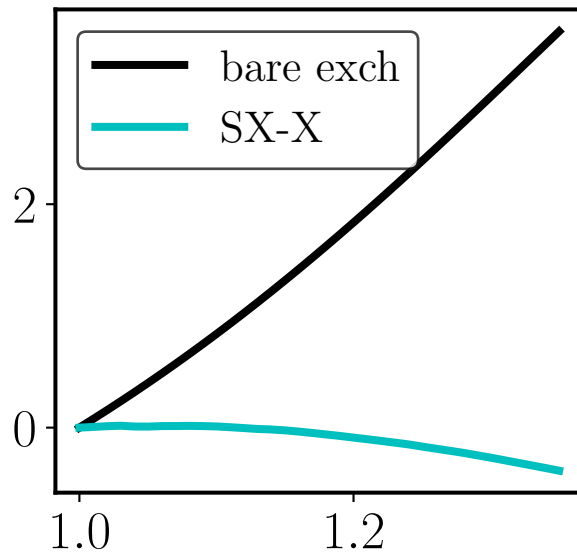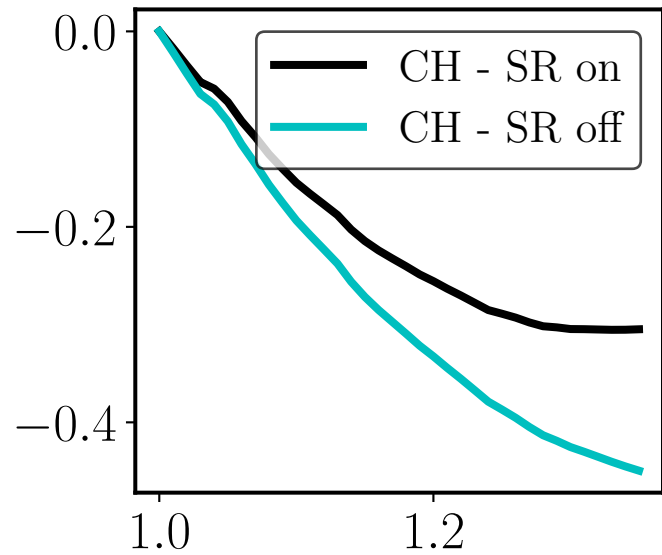

$R_{\text{CO}}$  (Å)

# band 3

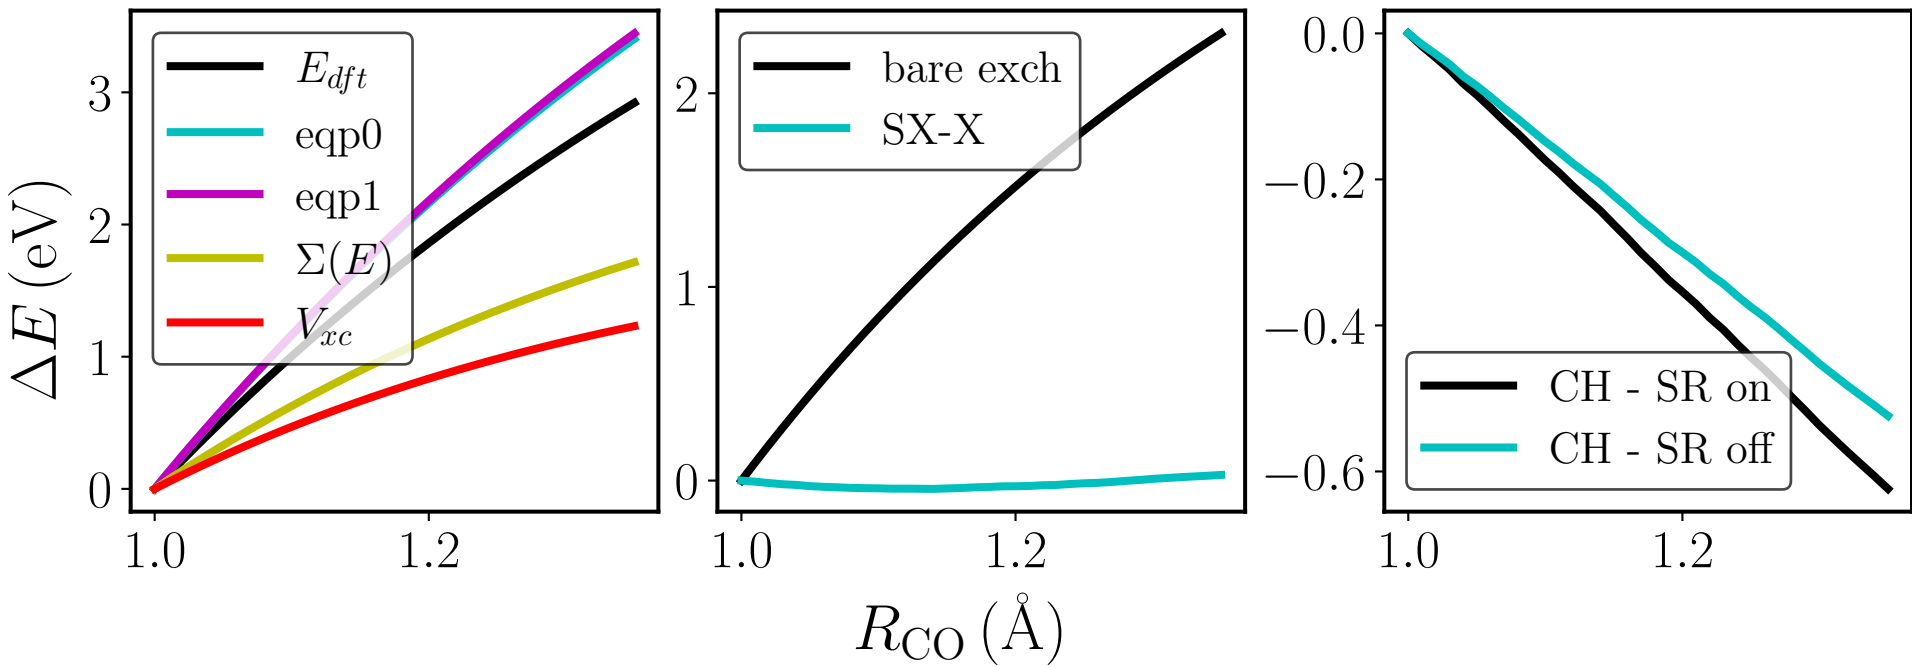

# band 4

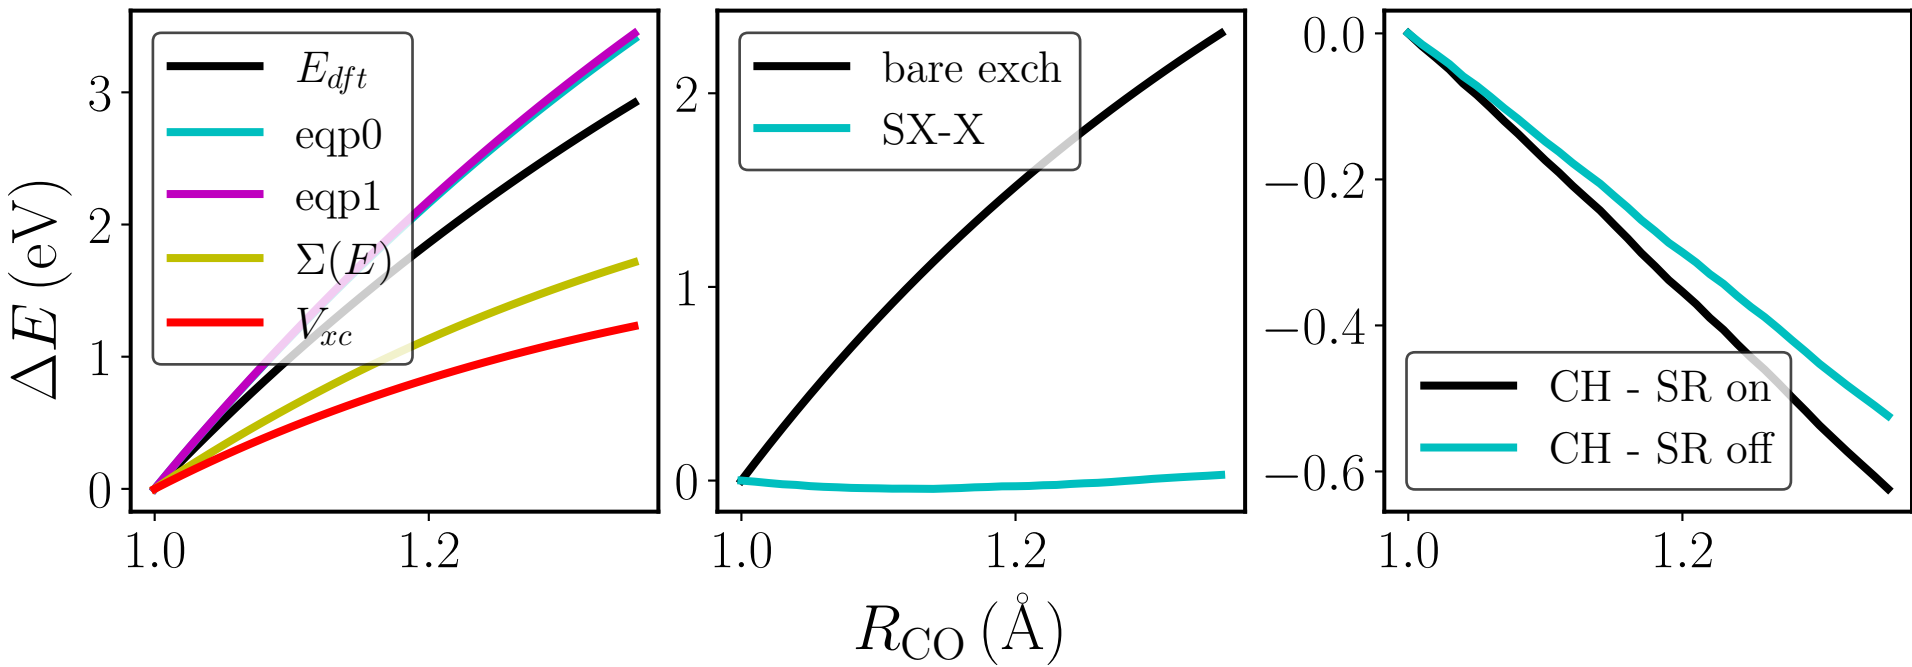

band 5

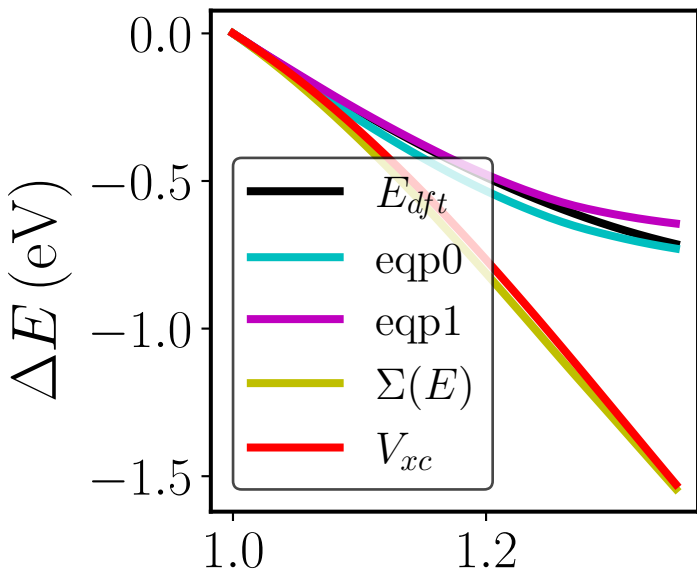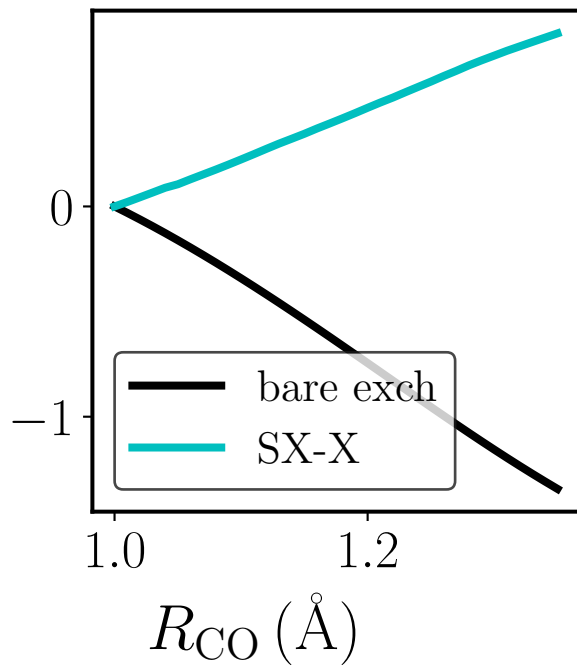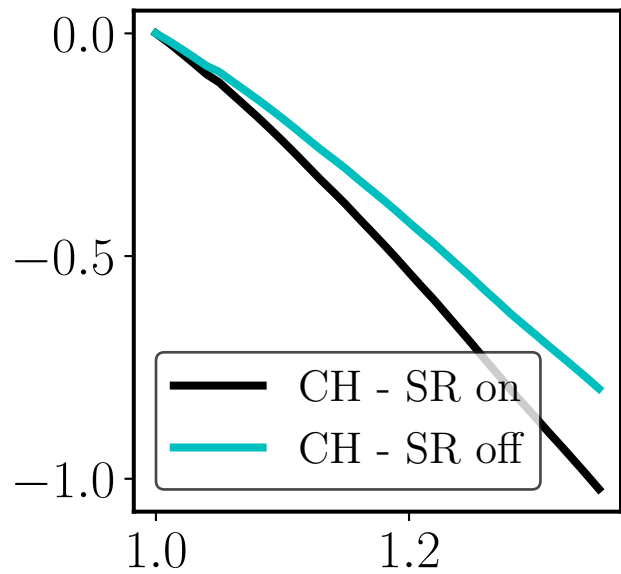

# band 6

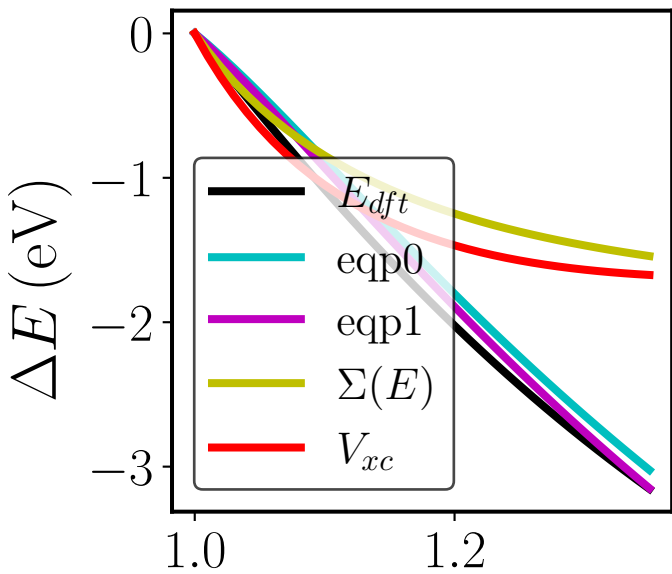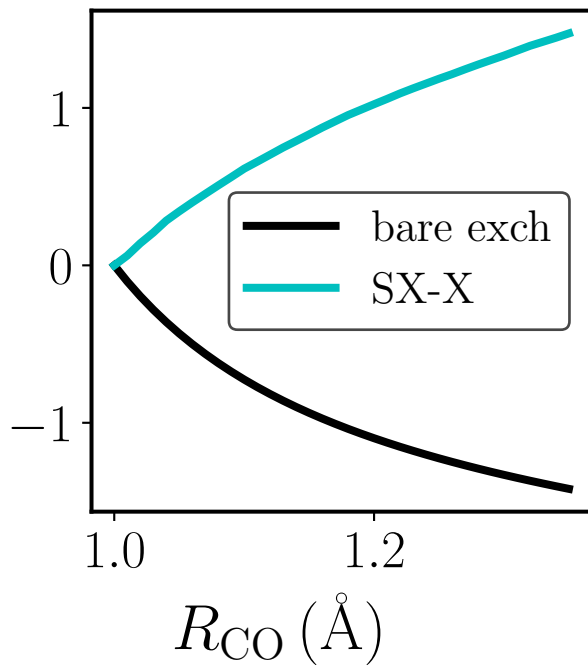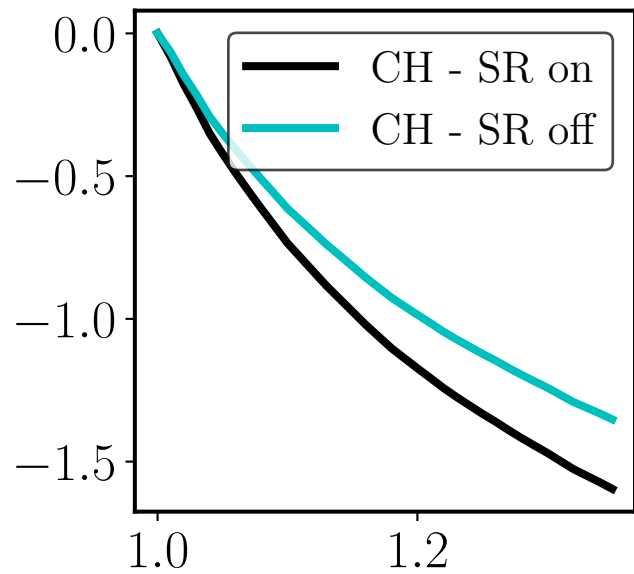

band 7

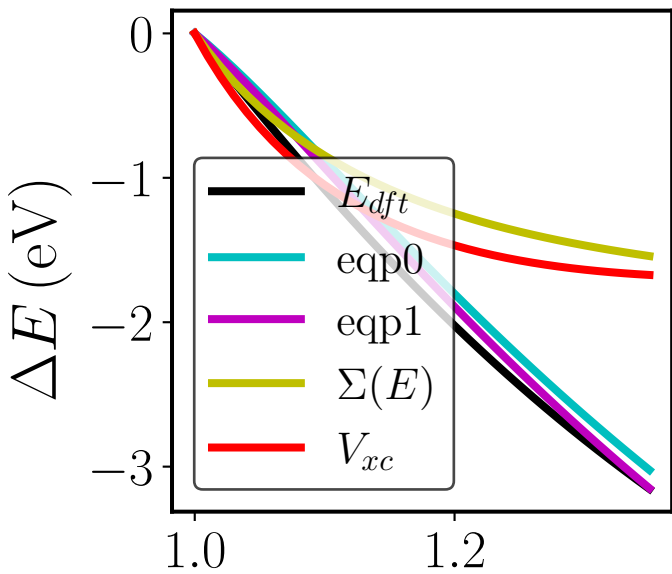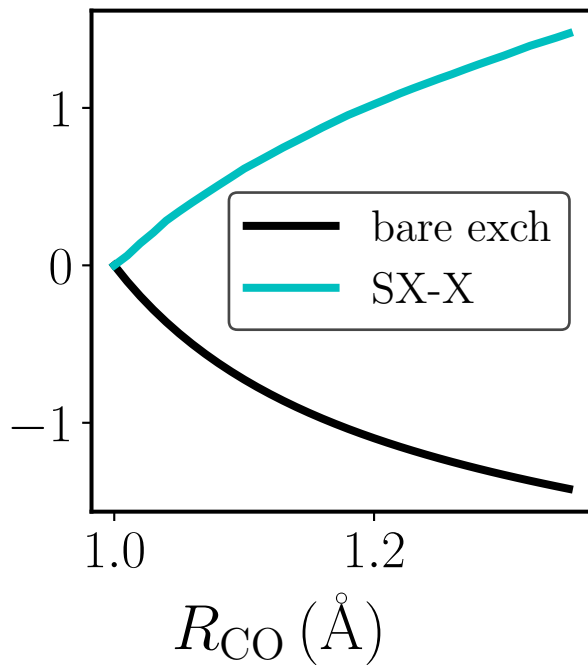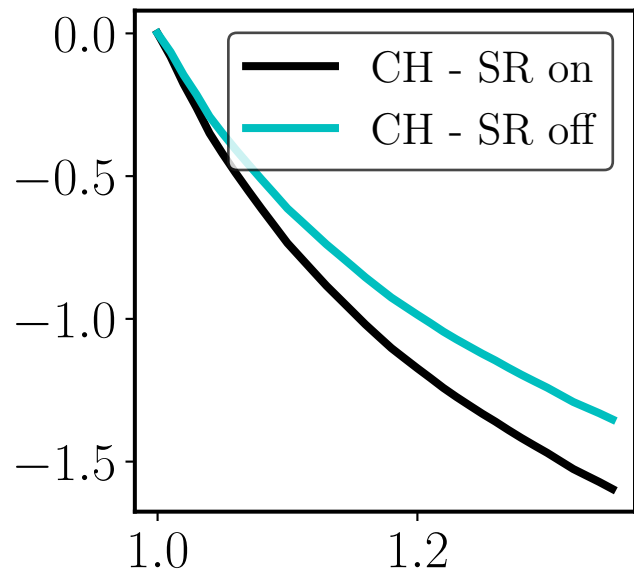

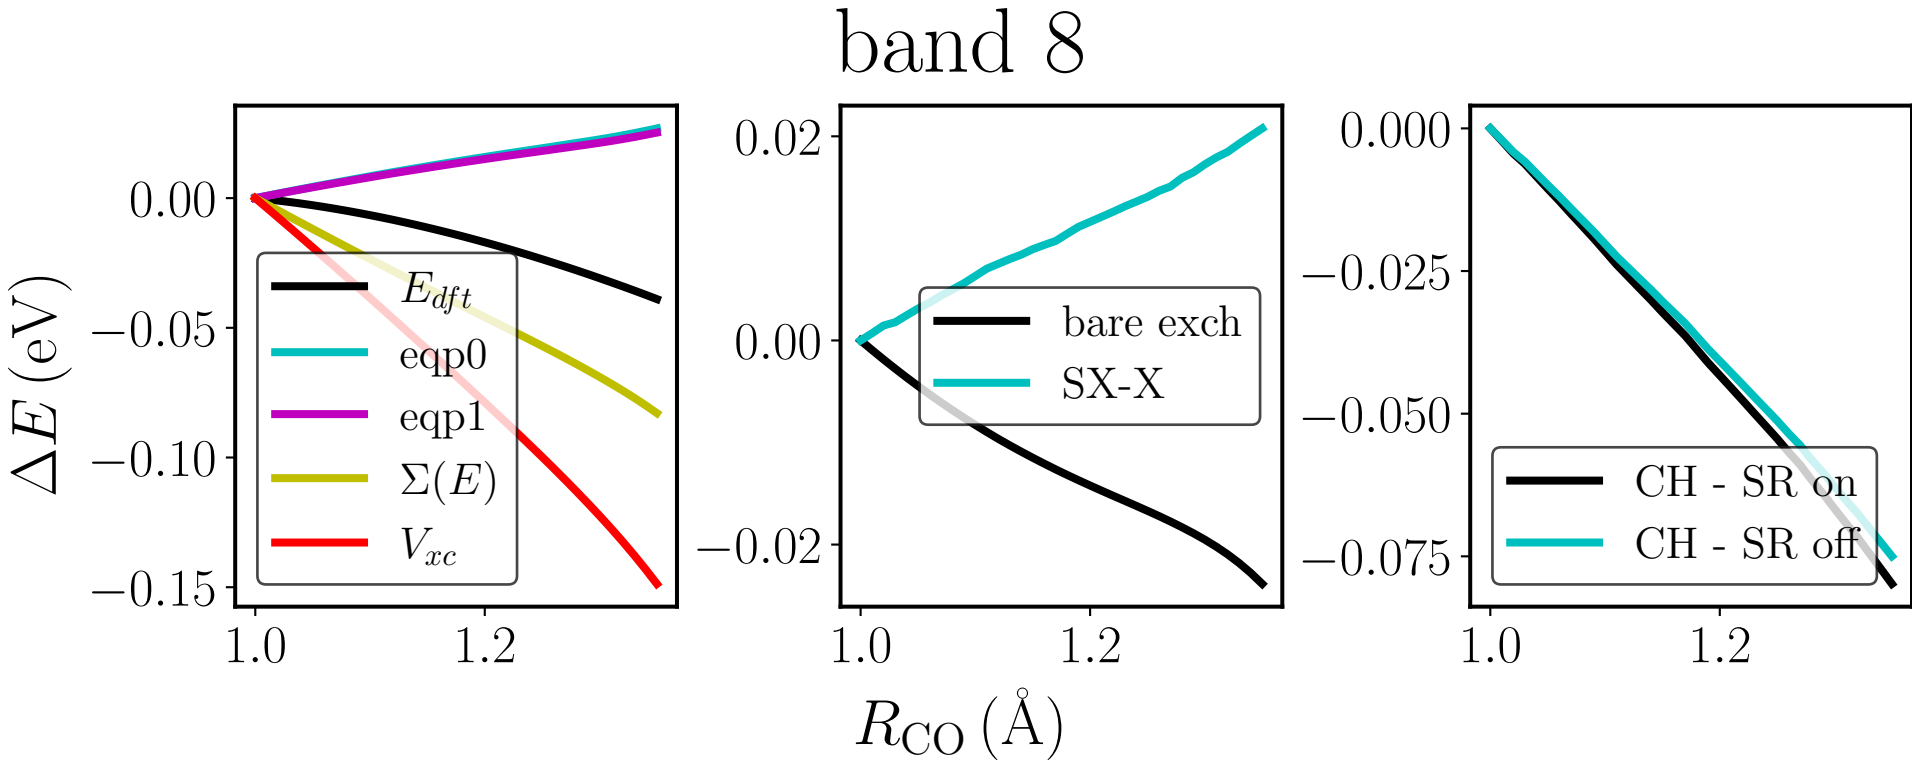



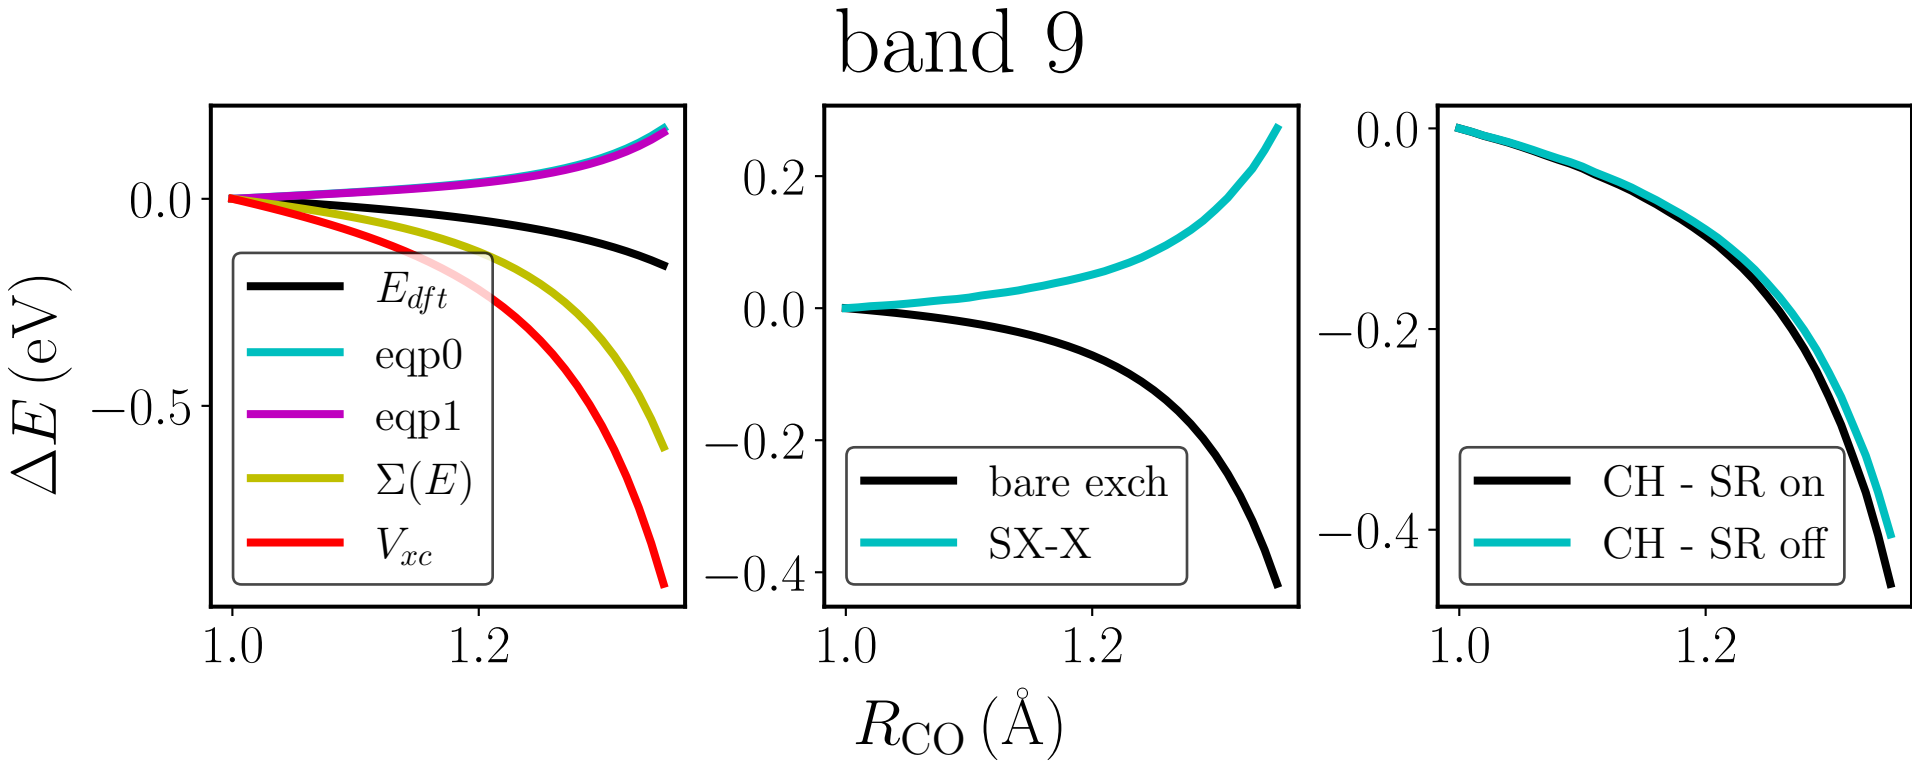

band 10

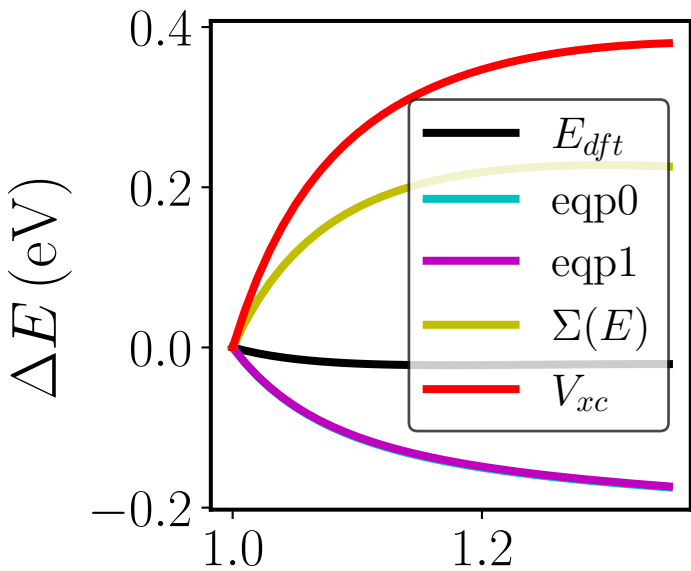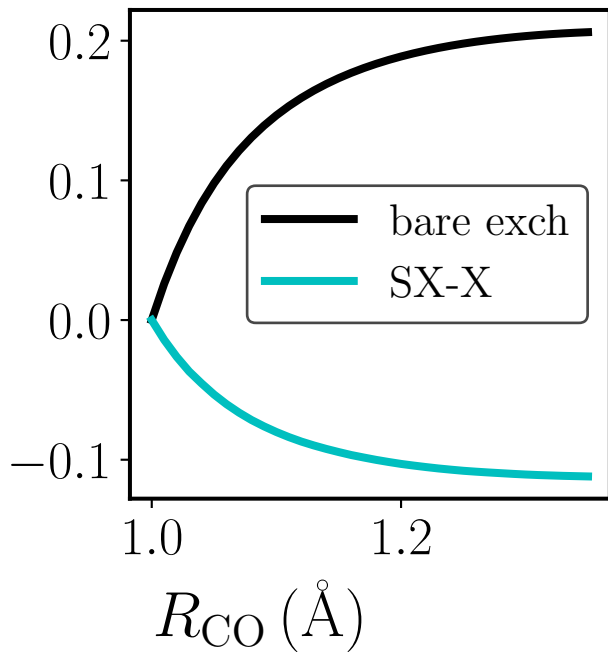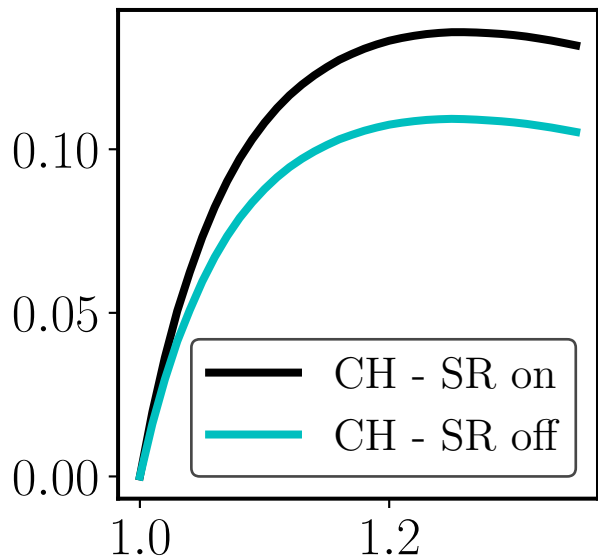

## band 11

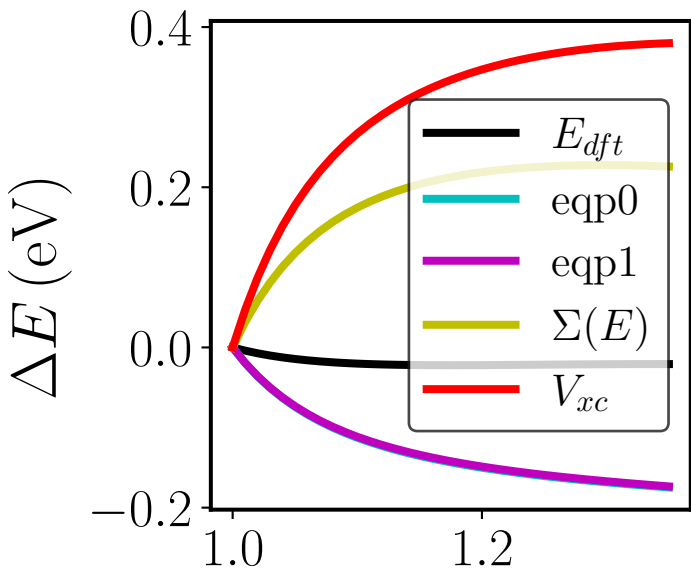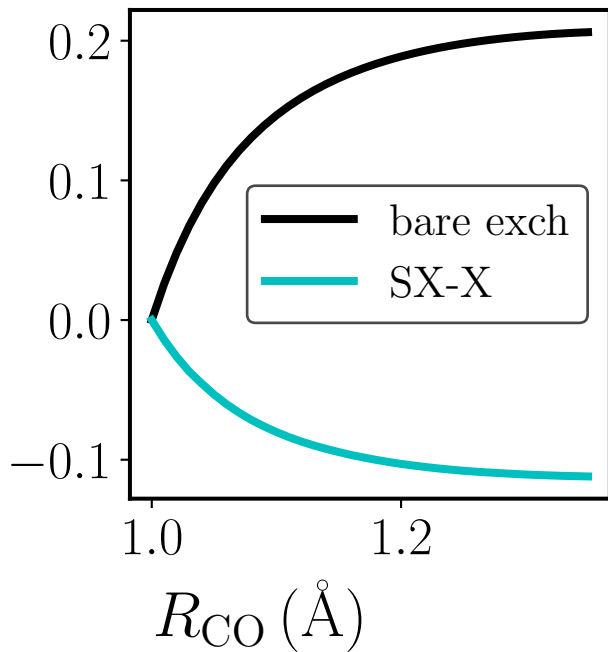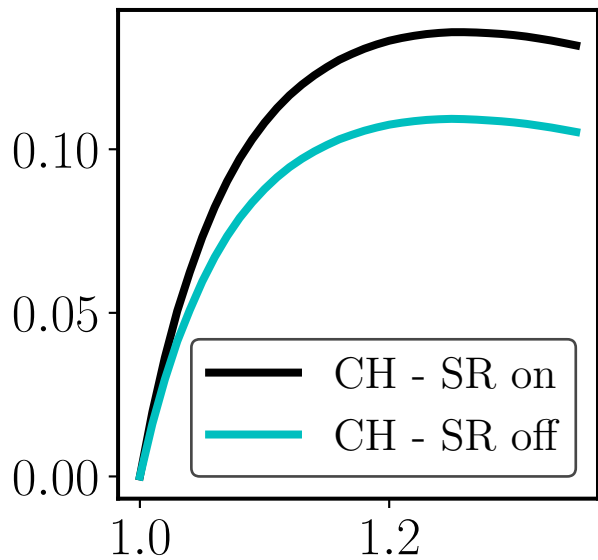

band 12

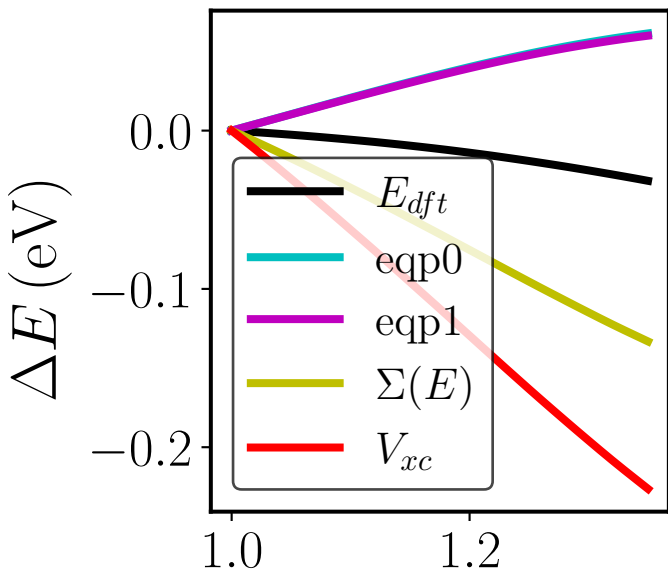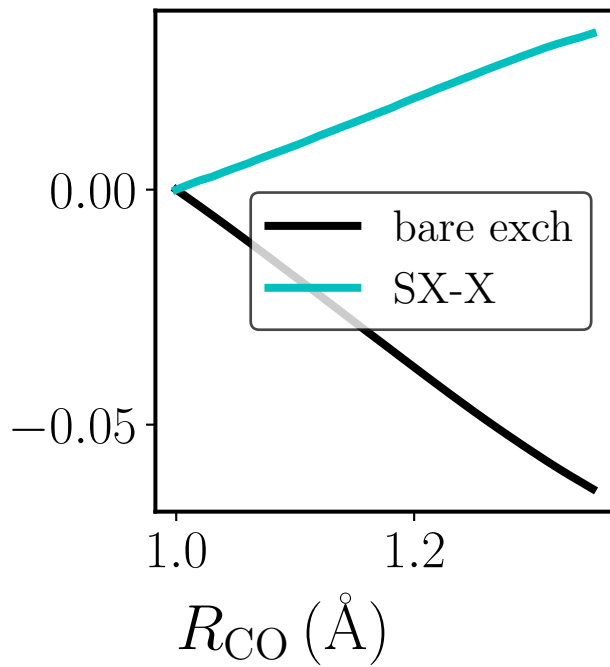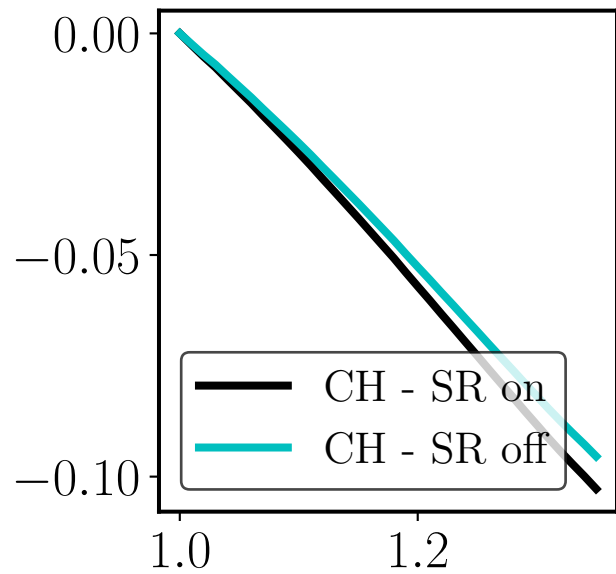

# band 13

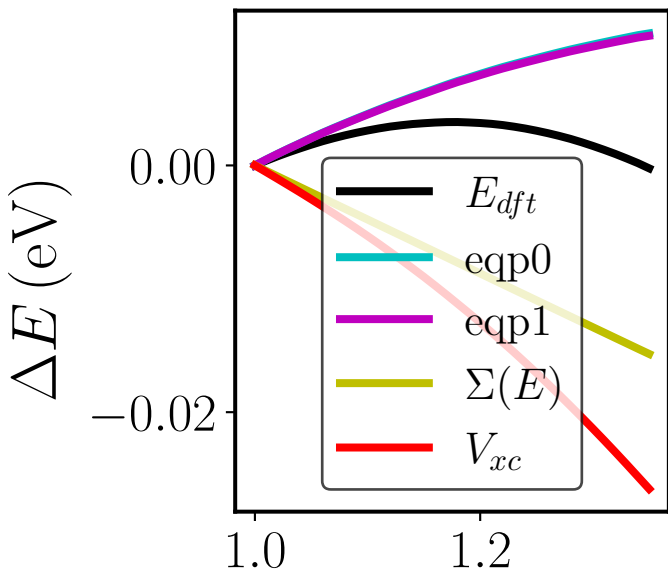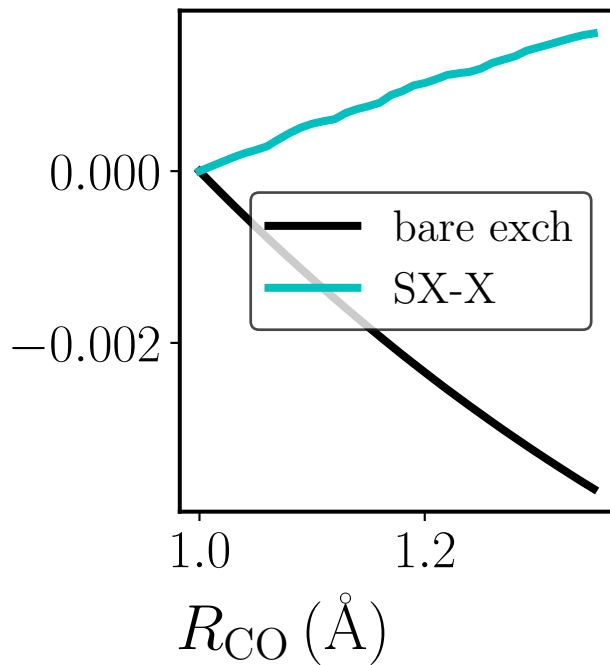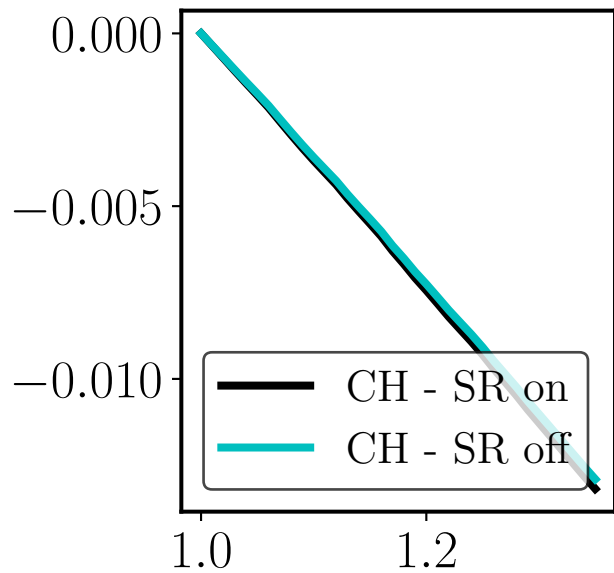

# band 14

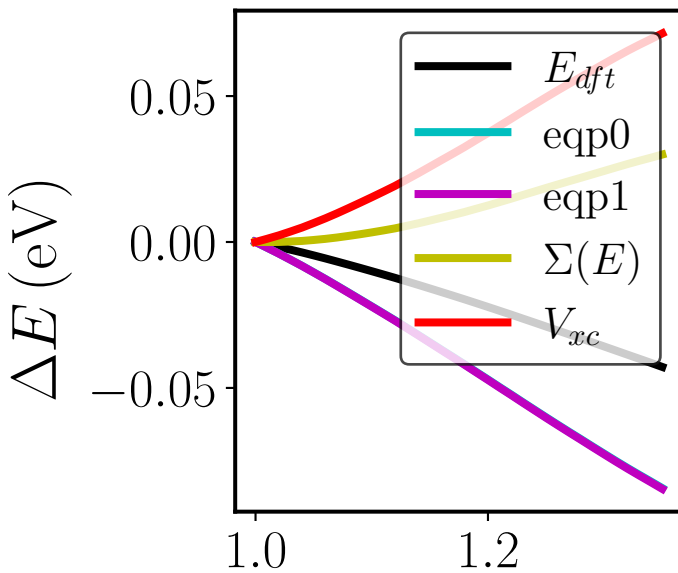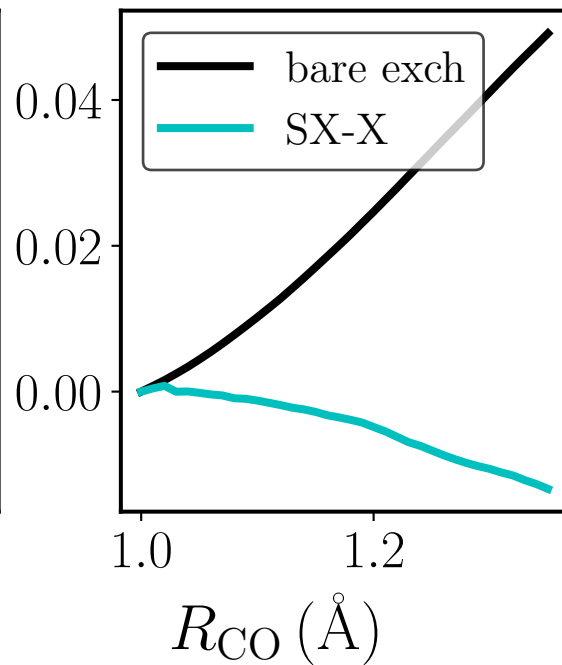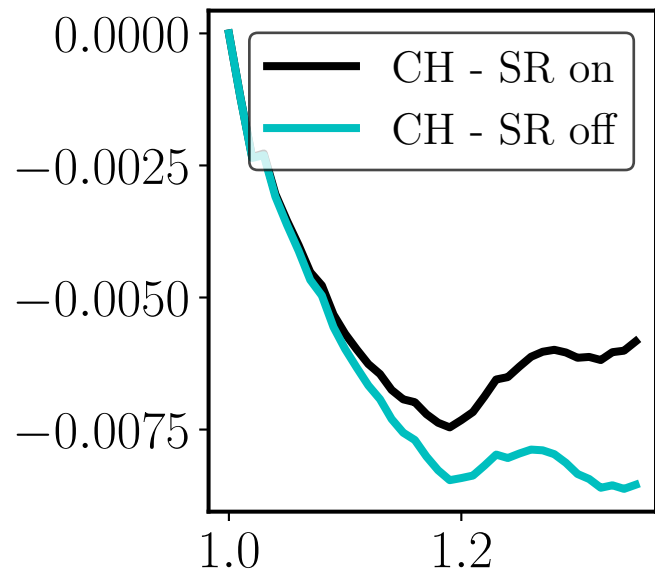

Supplement: Supplementary file 1 [file Energies_vs_Rco.pdf]
